# Supplementary material for: Anomalous Critical Slowdown at a First Order Phase Transition in Single Polymer Chains
Source: arXiv:1803.00770 source file (2018-03-02)
Supplement: Supplementary file 1 [file supplementary_material.pdf]

# Supplementary Material

## Anomalous Critical Slowdown at a First Order Phase Transition in Single Polymer chains

Shuangshuang Zhang,[1,2] Shuanhu Qi,[3] Leonid I. Klushin,[4]
Alexander M. Skvortsov,[5] Dadong Yan,[1] and Friederike Schmid[3]

[1] *Department of Physics, Beijing Normal University, Beijing 100875, China*
[2] *Graduate School Of Excellence Materials Science in Mainz, Staudingerweg 9, D-55128 Mainz, Germany*
[3] *Institut für Physik, Johannes Gutenberg-Universität Mainz, Staudingerweg 9, D-55099 Mainz, Germany*
[4] *Department of Physics, American University of Beirut, P. O. Box 11-0236, Beirut 1107 2020, Lebanon*
[5] *Chemical-Pharmaceutical Academy, Professora Popova 14, 197022 St. Petersburg, Russia*

**Brownian dynamic simulation scheme**

We adopt the over-damped Brownian dynamics to propagate the system. The system Hamiltonian is composed by two parts, i.e., $\mathcal{H} = \mathcal{H}_0 + \mathcal{H}_{\rm I}$, where $\mathcal{H}_0$ represents the contribution from the chain connection, while $\mathcal{H}_{\rm I}$ is the interaction part. To be more general we write the interaction part as a continuous integral

$$\mathcal{H}_{\rm I} = \frac{v}{2}\int d\mathbf{r}\hat{\rho}^2(\mathbf{r}) + \int d\mathbf{r} U_{\rm a}(\mathbf{r})\hat{\rho}(\mathbf{r}) \tag{1}$$

where the first term on the right hand side describes the excluded volume interaction, while the second term is adsorption energy. The above Hamiltonian corresponds to the system with pure adsorption, to include stretching, one could directly add the stretching force to the first bead. The density operator at present can be defined as a delta function $\hat{\rho}(\mathbf{r}) = \sum_j \delta(\mathbf{r} - \mathbf{R}_j)$, where the bead index $j$ runs over all beads. By performing the derivative and using the chain rule, we obtain

$$\frac{\partial \mathcal{H}}{\partial \mathbf{R}_j} = 3(2\mathbf{R}_j - \mathbf{R}_{j+1} - \mathbf{R}_{j-1}) + \frac{\partial}{\partial \mathbf{R}_j}\left[v\hat{\rho} + U_{\rm a}\right] \tag{2}$$

where $j$ is valid for any intermediate beads. The first bead $j = 1$ is only connected to the second bead, while for the last bead $j = N$, it is always fixed at the grafting point. By introducing a potential $\hat{\omega} \equiv v\hat{\rho} + U_{\rm a}$, the BD equation for the first bead is written as

$$\frac{d\mathbf{R}_1}{dt} = 3(\mathbf{R}_2 - \mathbf{R}_1) - \frac{\partial \hat{\omega}(\mathbf{R}_1)}{\partial \mathbf{R}_1} + \sqrt{2}\mathbf{f}_r, \tag{3}$$

for the bead $j = N$, $\frac{d\mathbf{R}_N}{dt} = 0$, for any bead $1 < j < N$

$$\frac{d\mathbf{R}_j}{dt} = 3(\mathbf{R}_{\rm j+1} + \mathbf{R}_{\rm j-1} - 2\mathbf{R}_{\rm j}) - \frac{\partial \hat{\omega}(\mathbf{R}_{\rm j})}{\partial \mathbf{R}_{\rm j}} + \sqrt{2}\mathbf{f}_r. \tag{4}$$

In order to proceed, we need an explicit expression for the potential derivative. Since the potential is directly determined by the bead density, the evaluation of its derivative is coupled to the way of assignment of particle-to-mesh density. In practice, we divide the simulation box uniformly into $n_{\rm x} \cdot n_{\rm y} \cdot n_{\rm z}$ cells. All the quantities are defined at the center of each cell, and we call these center points as mesh points. Each cell has a volume of $\Delta V = l_{\rm x} \cdot l_{\rm y} \cdot l_{\rm z}$. In the simulation we chose $l_{\rm x} = l_{\rm y} = l_{\rm z} = a$, meaning that each cell has a unit volume. Therefore the mesh points are located at $x = 0.5 + ml_{\rm x}$, $y = 0.5 + nl_{\rm y}$, $z = 0.5 + ol_{\rm z}$, where the integers $m \in [0, n_{\rm x} - 1]$, $n \in [0, n_{\rm y} - 1]$, $o \in [0, n_{\rm z} - 1]$. Fractions of a bead are assigned to its neighbouring mesh points according to the predefined assignment function $g(\mathbf{r})$ depending only on the distance between the particle and mesh point. Rather than choosing $g$ as a delta function in the continuum case, in practice $g$ has a finite width playing the role of a smear function (or coarse-graining function).

In terms of this assignment function, the density operator can be written as $\hat{\rho}(\mathbf{r}_\alpha) = \frac{1}{\Delta V}\sum_j g(|\mathbf{R}_j - \mathbf{r}_\alpha|)$, where $\mathbf{r}_\alpha$ denotes the position of the $\alpha$th mesh point. Now we can write $\mathcal{H}_{\rm I}$ in a discretized form

$$\mathcal{H}_{\rm I} = \frac{v}{2}\Delta V \sum_\alpha \hat{\rho}^2(\mathbf{r}_\alpha) - \Delta V \varepsilon \sum_\alpha U_{\rm a}(\mathbf{r}_\alpha)\hat{\rho}(\mathbf{r}_\alpha) \tag{5}$$

which is equivalent to the corresponding interaction energy in Eq.(1) in the main text as $\Delta V = 1$. Then the derivative of $\mathcal{H}_{\rm I}$ can be performed to get

$$\frac{\partial \mathcal{H}_{\rm I}}{\partial \mathbf{R}_j} = \frac{\partial \hat{\omega}}{\partial \mathbf{R}_j} = \sum_{\alpha} \hat{\omega}(\mathbf{r}_{\rm g}) \frac{\partial}{\partial \mathbf{R}_j} g(|\mathbf{R}_j - \mathbf{r}_\alpha|) \tag{6}$$

To perform the derivative of the assignment function, we need its explicit expression. For such a purpose, we consider the mesh in which $\mathbf{R}_j$ is located. There are totally eight vertexes for the mesh, and let $i, j, k$ denote the indices along $x, y, z$ directions, respectively. This means that $i = 0, j = 0, k = 0$ mark the vertex number 0 with coordinate $(0, 0, 0)$; $i = 0, j = 0, k = 1$ is the vertex number 1 with coordinate $(0, 0, l_z)$, $i = 0, j = 1, k = 0$ is the vertex number 2 with coordinate $(0, l_y, 0)$, and so on until $i = 1, j = 1, k = 1$ is the the vertex number 7 with coordinate $(l_x, l_y, l_z)$. Within this mesh, the $j$th bead is located at $\mathbf{R}_j = (X, Y, Z)$. There are several choices for the assignment function. The lowest order scheme is to assign each bead to its nearest mesh point, and this is called the nearest-grid-scheme. Here we use a higher order scheme, which assigns a fraction of bead to each of its eight nearest mesh points. The fraction assigned to a given vertex is proportional to the volume of a rectangle whose diagonal is the line connecting the particle position and the mesh point on the opposite side of the mesh cell. With the precise arrangement of vertexes, the assignment function for each vertex can be written as

$$\begin{aligned} & g(\mathbf{R}_j - \mathbf{r}_\alpha) \\ & = \frac{(l_x - |r_{\alpha x} - X|)(l_y - |r_{\alpha y} - Y|)(l_z - |r_{\alpha z} - Z|)}{l_x l_y l_z} \end{aligned} \tag{7}$$

where $g$ ranges from 0 to 7, $r_{g\alpha}$ is the $\alpha$ component of $\mathbf{r}_g$. Performing the derivative of the assigning function directly, we obtain

$$\begin{aligned} \frac{\partial \hat{\omega}}{\partial R_{jx}} = & \frac{\hat{\omega}(\mathbf{r}_4) - \hat{\omega}(\mathbf{r}_0)}{l_x} \frac{(l_y - Y)(l_z - Z)}{l_y l_z} \\ & + \frac{\hat{\omega}(\mathbf{r}_5) - \hat{\omega}(\mathbf{r}_1)}{l_x} \frac{(l_y - Y)Z}{l_y l_z} \\ & + \frac{\hat{\omega}(\mathbf{r}_6) - \hat{\omega}(\mathbf{r}_2)}{l_x} \frac{Y(l_z - Z)}{l_y l_z} + \frac{\hat{\omega}(\mathbf{r}_7) - \hat{\omega}(\mathbf{r}_3)}{l_x} \frac{YZ}{l_y l_z}, \end{aligned} \tag{8}$$

$$\begin{aligned} \frac{\partial \hat{\omega}}{\partial R_{jy}} = & \frac{\hat{\omega}(\mathbf{r}_2) - \hat{\omega}(\mathbf{r}_0)}{l_y} \frac{(l_x - X)(l_z - Z)}{l_x l_z} \\ & + \frac{\hat{\omega}(\mathbf{r}_6) - \hat{\omega}(\mathbf{r}_4)}{l_y} \frac{X(l_z - Z)}{l_x l_z} \\ & + \frac{\hat{\omega}(\mathbf{r}_3) - \hat{\omega}(\mathbf{r}_1)}{l_y} \frac{(l_x - X)Z}{l_x l_z} + \frac{\hat{\omega}(\mathbf{r}_7) - \hat{\omega}(\mathbf{r}_5)}{l_y} \frac{XZ}{l_x l_z}, \end{aligned} \tag{9}$$

and

$$\begin{aligned} \frac{\partial \hat{\omega}}{\partial R_{jz}} = & \frac{\hat{\omega}(\mathbf{r}_1) - \hat{\omega}(\mathbf{r}_0)}{l_z} \frac{(l_x - X)(l_y - Y)}{l_x l_y} \\ & + \frac{\hat{\omega}(\mathbf{r}_5) - \hat{\omega}(\mathbf{r}_4)}{l_z} \frac{X(l_y - Y)}{l_x l_y} \\ & + \frac{\hat{\omega}(\mathbf{r}_3) - \hat{\omega}(\mathbf{r}_2)}{l_z} \frac{(l_x - X)Y}{l_x l_y} + \frac{\hat{\omega}(\mathbf{r}_7) - \hat{\omega}(\mathbf{r}_6)}{l_z} \frac{XY}{l_x l_y}. \end{aligned} \tag{10}$$

Inserting the above expressions to the BD equation gives the final form which we use in our BD simulations.

There are two remarks. First, a bead located at $z \leq 0.5$ contributes density only to the 4 nearest mesh points due to the impenetrable boundary condition. This indicates that any bead at $z < 0.5$ acts like it is at $z = 0.5$. Second, the adsorption potential is usually defined as a steplike function with the potential width the segmental length $a$ ($a \equiv 1$ is the unit length). This means that $U_{\rm a}(z) = -\varepsilon$ for $z < 1$ and zero otherwise. In the present case, however, we introduce an assignment function to distribute density to the nearest mesh points, which means that a bead can still feel the force even it is at a location with $z > 1$. Considering the specific form of the assignment function, the apparent potential imposed on a bead should be regulated as $U_{\rm a}(\mathbf{r}) = -\varepsilon \min(1, 3/2 - z)$ for $z < 3/2$, and zero otherwise.

**Hard wall vs. logarithmic potentials**

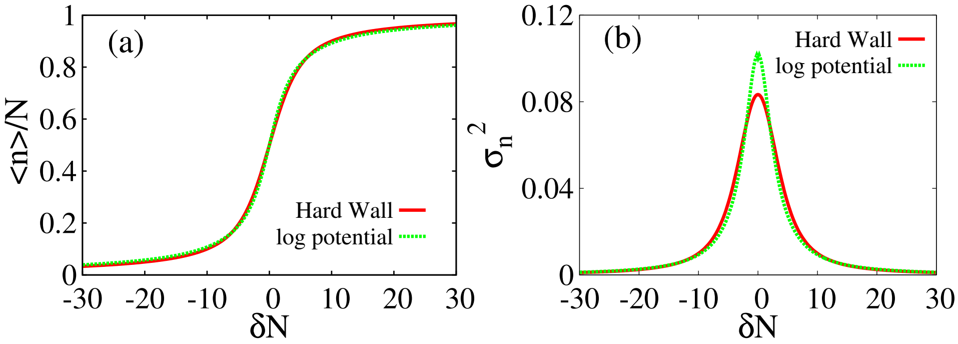


FIG. 1. Comparison of the normalized mean position of the boundary (a) and its fluctuations (b) for the effective Hamiltonian with hard wall boundaries and with logarithmic potentials. The control parameter is the product $\delta N$.

The logarithmic wall model used in our paper has the advantage of generating tractable results for the most probable value of the interface position $\bar{n}$, and its fluctuations, $\sigma^2(n)$, evaluated in the harmonic approximation, see Eqs. (3),(4)) in the main text. In contrast to this, with the more physically meaningful hard wall boundaries the position of the minimum always coincides with one of the boundaries (except for the transition point itself), and the fluctuations are essentially non-Gaussian. Hence, there is no simple way to describe the boundary dynamics. The partition function of the hard wall model is given by:

$$Q(\delta, N) = \int_0^N \exp(\delta\, n)\, d\, n = \exp\left(\frac{\delta\, N}{2}\right) \frac{\sinh\left(\frac{\delta\, N}{2}\right)}{\delta} \tag{11}$$

which leads to the average $\langle n \rangle = \frac{\partial \log Q}{\partial \delta}$ and fluctuations $\sigma_{\rm n}^2 = \frac{\partial^2 \log Q}{\partial \delta^2}$ in the following form:

$$\langle n \rangle = \frac{N}{2}\left(1 + \coth\left(\frac{\delta\, N}{2}\right) - \frac{2}{\delta\, N}\right) \tag{12}$$

$$\sigma_{\rm n}^2 = \frac{N^2}{4}\left(\left(\frac{2}{\delta\, N}\right)^2 - \sinh^{-2}\left(\frac{\delta\, N}{2}\right)\right) \tag{13}$$

Fig. 1 shows the comparison of the normalized average $\langle n \rangle$ and the most probable value $\bar{n}$ , as well as the corresponding normalized fluctuations for models with hard wall and logarithmic potentials. In the latter, the amplitude is chosen to minimize the overall discrepancy, $A = \sqrt{3/2}$.

**Solving the Langevin equation with multiplicative noise**

In the main manuscript, we have replaced the variable diffusion constant $D(n)$ by an effective constant diffusion constant $D(n^*)$ for simplicity. However, we can also keep the variable constant $D(n)$, and obtain similar results. At variable $D(n)$, the noise also becomes dependent of $n$, i.e., multiplicative, which induces drift. To remove this problem, we transform the Langevin equation into one with additive noise *via* the variable transform $\mathrm{d}n \to \mathrm{d}\tilde{n} = \mathrm{d}n/\sqrt{D(n)}$, giving $\dot{\tilde{n}} = \tilde{f}(\tilde{n}) + \sqrt{2}\,\xi$. The effective "driving force" term $\tilde{f}(\tilde{n})$ must be chosen such that $n$ is Boltzmann distributed with the Hamiltonian $\mathcal{H}_{\rm eff}$ (Eq. (2)), i.e., $\tilde{f}(\tilde{n}) = -\partial_{\tilde{n}} E(\tilde{n})$ with

$$E(\tilde{n}) = \mathcal{H}_{\rm eff}(n) + \log(\mathrm{d}\tilde{n}/\mathrm{d}n). \tag{14}$$

The characteristic time scale is dominated by the diffusive process around the minimum $\tilde{n}^*$ of $E$, and evolution of $\tilde{n}$ is approximated by the Ornstein-Uhlenbeck process, which has the inverse relaxation time [1] given by

$$\tau_n^{-1} = \frac{\partial^2}{\partial \tilde{n}^2} E(\tilde{n})|_{\tilde{n}^*} = D(n^*) \frac{\partial^2}{\partial n^2}(\mathcal{H}_{\rm eff}(n) - \frac{1}{2}\log D(n))\Big|_{n^*}. \tag{15}$$

where $n^*$ is the root of the equation $\frac{\partial}{\partial n}(\mathcal{H}_{\rm eff}(n) - \frac{1}{2}\log D(n)) = 0$. With the diffusion coefficient given by Eq.(9) of the Letter this becomes a cubic equation:

$$2An(s+n) - 2A(N-n)(s+n) + n(N-n) - 2\delta n(s+n)(N-n), \tag{16}$$

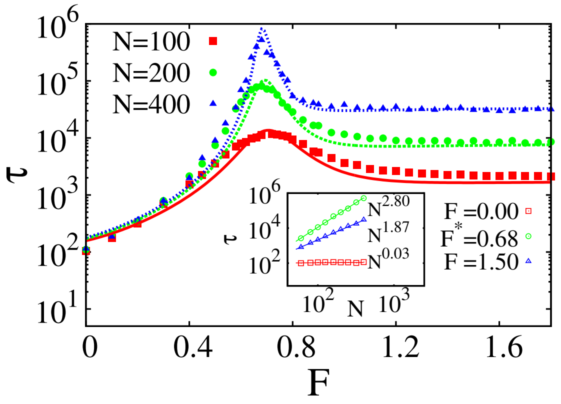


FIG. 2. Characteristic relaxation time $\tau$ of free end correlations vs. stretching force for chain lengths $N = 100, 200, 400$ at $-\varepsilon = 0.80$. Symbols are data from BD simulations, and lines correspond to the prediction based on the dynamic model with a rigorous treatment of the variable diffusion coefficient. Fitting parameters are $\alpha = 0.1$, $\zeta_{\rm ads} = 3.0$

where $s = \frac{\zeta_{\rm ads}}{\alpha\zeta_0}$. The average relaxation time for the free end height evaluated with the help of Eq. (15) with $\alpha = 0.1$, $\zeta_{\rm ads} = 3.0$ is shown in comparison with the simulations data in Fig. 2. The quality of the fit is very close to that of the simplified treatment presented in the letter, although the best values of the fitting parameters differ.

[1] H. Risken, *The Fokker-Planck equation*, Springer Series in Synergetics, Vol. 18, Springer, 1996
